# Supplementary material for: Effective Targeted Attacks for Adversarial Self-Supervised Learning
Source: arXiv:2210.10482 source file (2023-10-26)
Supplement: Supplementary file 1 [file appendix_influence.tex]

\begin{wrapfigure}[11]{r}{0.5\textwidth}
    \vspace{-0.13in}
    \centering
    
    \begin{subfigure}[t]{0.43\linewidth}
        \centering
        \includegraphics[width=\linewidth]{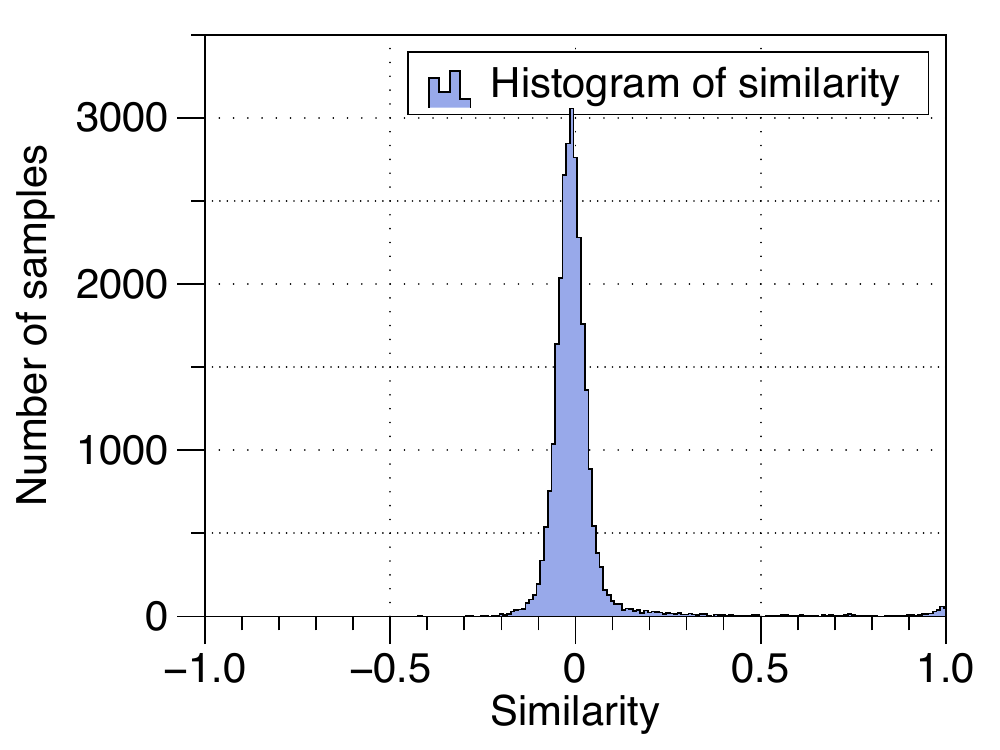}
        \caption{Histogram of cosine similarity between sampled pairs.}
        \vspace{-0.1in}
    \end{subfigure}
    
    \begin{subfigure}[t]{0.43\linewidth}
        \centering
        \includegraphics[width=\linewidth]{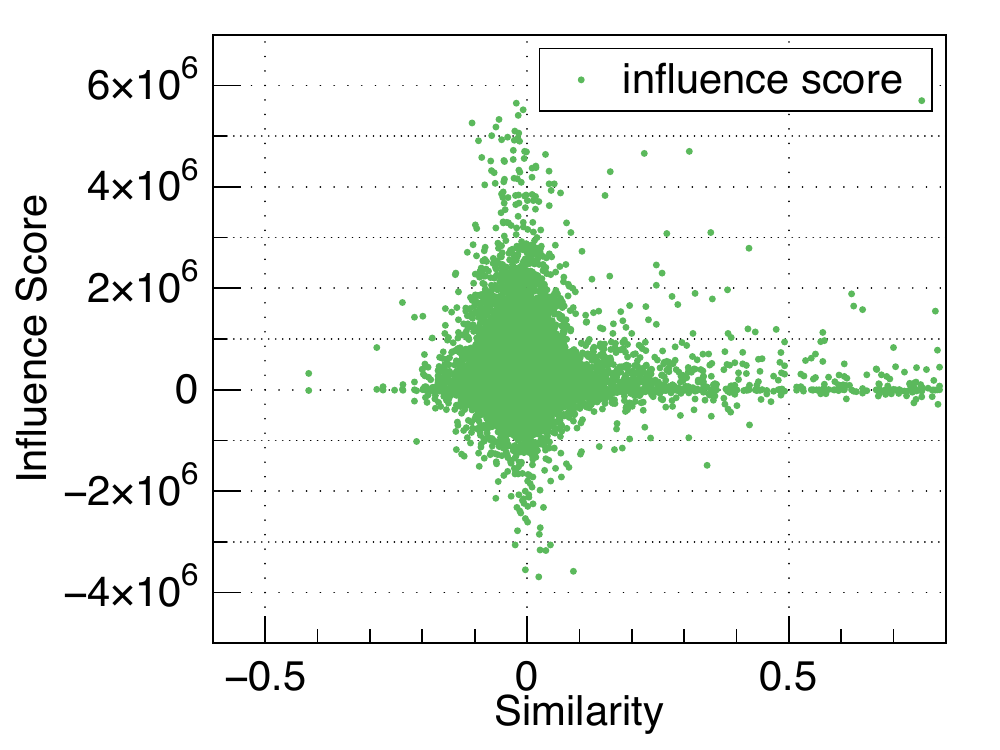}
        \caption{Scatter of influence score based on similarity.}
    \end{subfigure}
    
    \caption{Analysis with influence score.}
    \label{appendix:influence}
\end{wrapfigure}
