# Supplementary material for: Effective Targeted Attacks for Adversarial Self-Supervised Learning
Source: arXiv:2210.10482 source file (2023-10-26)
Supplement: Supplementary file 2 [file appendix_table_rFT.tex]

\begin{table}[h]
\caption{Experimental results against white box attacks on ResNet18 trained on the CIFAR10. We evaluate adversarial SSL with robust finetuning. Clean is the accuracy of clean images. All models are evaluated with PGD $\ell_{\infty}$ with 20 steps of $\epsilon=$ 0.0314 and AutoAttack~\citep{croce2020AA}. Untargeted attack maximizes the training loss between the differently augmented but the same instances to generate adversaries. To see the effectiveness of our methods, we test TAROSS on positive-only SSL, i.e., BYOL, SimSiam (grey box).}
\centering
\begin{adjustbox}{width=\textwidth}
\label{appendix:rFT}
\centering
  \begin{tabular}{cghggg} %
    \toprule
    \rowcolor{white}
    {Train type}&{Self-supervised framework}&{Method}&{Clean} &PGD $\ell_{\infty}$& AutoAttack\\
    %Train Type&Method&Clean&AutoAttack &PGD $\ell_{\infty}$ &PGD $\ell_2$ &PGD $\ell_1$\\
    \midrule 
    \rowcolor{white}
    \multirow{6}{*}{\makecell{Robust Fine tuning}} &
    {SimCLR}&RoCL~\citep{kim2020rocl}&78.14&42.89&27.19\\
    \rowcolor{white}
    {}&{SimCLR}&ACL~\citep{jiang2020ACL}&79.96&39.37&35.97\\
    {}& {BYOL}&Untargeted attack&72.65	&16.20	&0.01\\
    {}&{BYOL}&\textbf{TAROSS}&\textbf{84.52}&	\textbf{31.19}&	\textbf{21.01}\\
    {}&{SimSiam}&Untargeted attack&69.69&41.49&32.41\\
    {}&{SimSiam}&\textbf{TAROSS}&\textbf{78.47} & \textbf{42.22}&\textbf{36.32}\\
    \bottomrule
  \end{tabular}
  \end{adjustbox}
\end{table}
