# Supplementary material for: Effective Targeted Attacks for Adversarial Self-Supervised Learning
Source: arXiv:2210.10482 source file (2023-10-26)
Supplement: Supplementary file 3 [file supple_table3.tex]

\begin{table}[t]
\caption{\small Experimental results with white box attacks on ResNet18 trained on the CIFAR-100. Clean is the accuracy of clean images. All models are trained with $\ell_{\infty}$; thus the $\ell_{\infty}$ is the \emph{seen} adversarial attack.}
\centering
  \begin{tabular}{lcccc} %
    \toprule
    Method& Clean & AA &PGD $\ell_{\infty}$\\
    \midrule
    \multicolumn{3}{l}{\small{Self-supervised linear evaluation}}
    \\
    RoCL~\cite{kim2020rocl}\\
    ACL~\cite{jiang2020ACL}\\
    \textbf{Ours}\\
    \midrule
    \multicolumn{3}{l}{\small{Self-supervised robust linear evaluation}}
    \\
    RoCL~\cite{kim2020rocl}\\
    ACL~\cite{jiang2020ACL}\\
    Ours &\\
    \bottomrule
  \end{tabular}
\end{table}
